# Supplementary material for: How to Agree to Disagree: Managing Ontological Perspectives using Standpoint Logic
Source: arXiv:2206.06793 source file (2022-08-01)
Supplement: Supplementary file 1 [file appendix.tex]

\appendix

\subsection{Proof Theory}\label{sec-sub:proof-theory}

Systems of modal logic are normally described via their axiomatic presentation, and in this spirit we now give a Hilbert-style axiomatic proof system for $\PropStandpointLogic$. %We specify a set of axioms, which capture significant aspects of the semantics, and four standard inference rules.
We write $\vdash_{\PropStandpointLogic} \phi$ to mean that $\phi$ is
a derivable theorem of $\PropStandpointLogic$ (i.e. $\phi$ is derivable from no premises).
% The axioms are specified by schemas, where all occurrences of
% each of the meta-variables ($\phi$ and $\psi$) may be instantiated by
% any formula of $\PropStandpointLang$ (all occurrence of a given meta-variable must be substituted by the same formula, but where both $\phi$ and $\psi$
% occur in a schema they may be substituted by different formulas).

Since standpoint logic is built upon an underlying classical logic,
all classically valid formulas are theorems, and we assume that we have 
a method for determining them.
In addition, $\PropStandpointLogic$\ satisfies the following
axioms:

\begin{enumerate}[series=axioms,label={\bf A\arabic*.},ref={\bf A\arabic*},leftmargin=2em,labelwidth=3em] 
	\item[\ak] $\standbs (\phi\imp \psi) \imp (\standbs  \phi \imp \standbs  \psi) $ \label{AX:K}
	\item[\ad] $\standbs  \phi \imp  \standds\phi$\label{AX:D}
	\item[\at] $\allstandb \phi \imp \phi $ (only applies to the universal operator $\allstandb$.)
	
	\item[\asfour] $\standbs  \phi \imp \standbsp  \standbs  \phi$\label{AX:4}
	
	\item[\asfive] $\standds \phi \imp \standbsp \standds \phi$\label{AX:5}
	
	\item[{\bf AP}] $(\standbs  \phi \imp \standbsp \phi)\dimp(\sp \preceq s)$\label{AX:P}
\end{enumerate}

%	Thus, each operator $\standbs$ obeys the axioms \ak,  \ad, {\bf 4} and  {\bf 5}, which are the standard axioms for the normal modal logic {\bf KD45}, and the $\allstandb$ operator satisfies an \sfive modality.% This is discussed in more detail in section \ref{SEC:CH4-axioms-45}.

The  inference  rules  of  $\PropStandpointLogic$ are the standard for modal logic: 
classical  theorems are provable ({\bf  RC}), all instances of the axioms are provable ({\bf RA}), the  classical \emph{modus ponens\/} ({\bf MP}), and the rule of necessitation (\rn).
\iffalse
\begin{enumerate}[leftmargin=2em,labelwidth=3em] 
	\item[\bf RC.] $\vdash_\PropStandpointLogic \phi$, if $\phi$ is a
	theorem of classical propositional
	logic (where we treat all modal sub-formulas of $\phi$ 
	as atomic propositions).
	
	\item[\bf RA.] $\vdash_\PropStandpointLogic \phi$, if $\phi$ is
	an instance of one of the modal axioms (\ak, \ad, \at,
	\asfour, \asfive).
	
	\item[{\bf MP.}] If $\vdash_\PropStandpointLogic \phi$ 
	and  $\vdash_\PropStandpointLogic \phi\imp \psi$,
	then  $\vdash_\PropStandpointLogic  \psi$.
	\label{AxNec}
	
	\item[{\bf RN.}] If $\vdash_\PropStandpointLogic \phi$, 
	then  $\proveSo \standbs \phi$,
	for all
	standpoints $s\in S$.
	\label{AxNec}
\end{enumerate}
\fi

A \emph{proof\/} of $\phi$ in $\PropStandpointLogic$ is a sequence of
formulas, ending in $\phi$, such that each formula is either provable directly
by {\bf RC} or {\bf RA}, or is derivable using {\bf MP} or \rn
from formulas that occur earlier in the sequence.
